# Supplementary material for: Semi-supervised Learning with the EM Algorithm: A Comparative Study between Unstructured and Structured Prediction
Source: arXiv:2008.12442 source file (2020-08-28)
Supplement: Supplementary file 1 [file appendix.tex]

\clearpage
\section*{Appendix}
This appendix shows empirical evaluation results on the Hurricane Mathew flood in North Carolina. Figure~\ref{fig:EMNOElevmuSigmaap},~\ref{fig:EMmuSigmaap}, and~\ref{fig:HMTmuSigmaap} show the parameter iterations of model parameters in unstructured EM without elevation, unstructured EM with elevation feature, and structured EM respectively. The overall trends look similar to the results on the Harvey dataset. The corresponding class posterior probabilities of pixels in three methods are shown in Figure~\ref{fig:EMNOelevPosterProbap},~\ref{fig:EMwithelevPosterProbap}, and~\ref{fig:HMTPosterProbap}. Comparison on class predictions are shown in Table~\ref{tab:comp1ap} and Figure~\ref{fig:predresultap}.

% \subsection{Parameter Iteration and Convergence (second dataset)}

\begin{figure}[ht]
\centering
\subfloat[Iteration of parameter $\boldsymbol{\mu}$]{%
      \includegraphics[height=1.7in,width=1.8in]{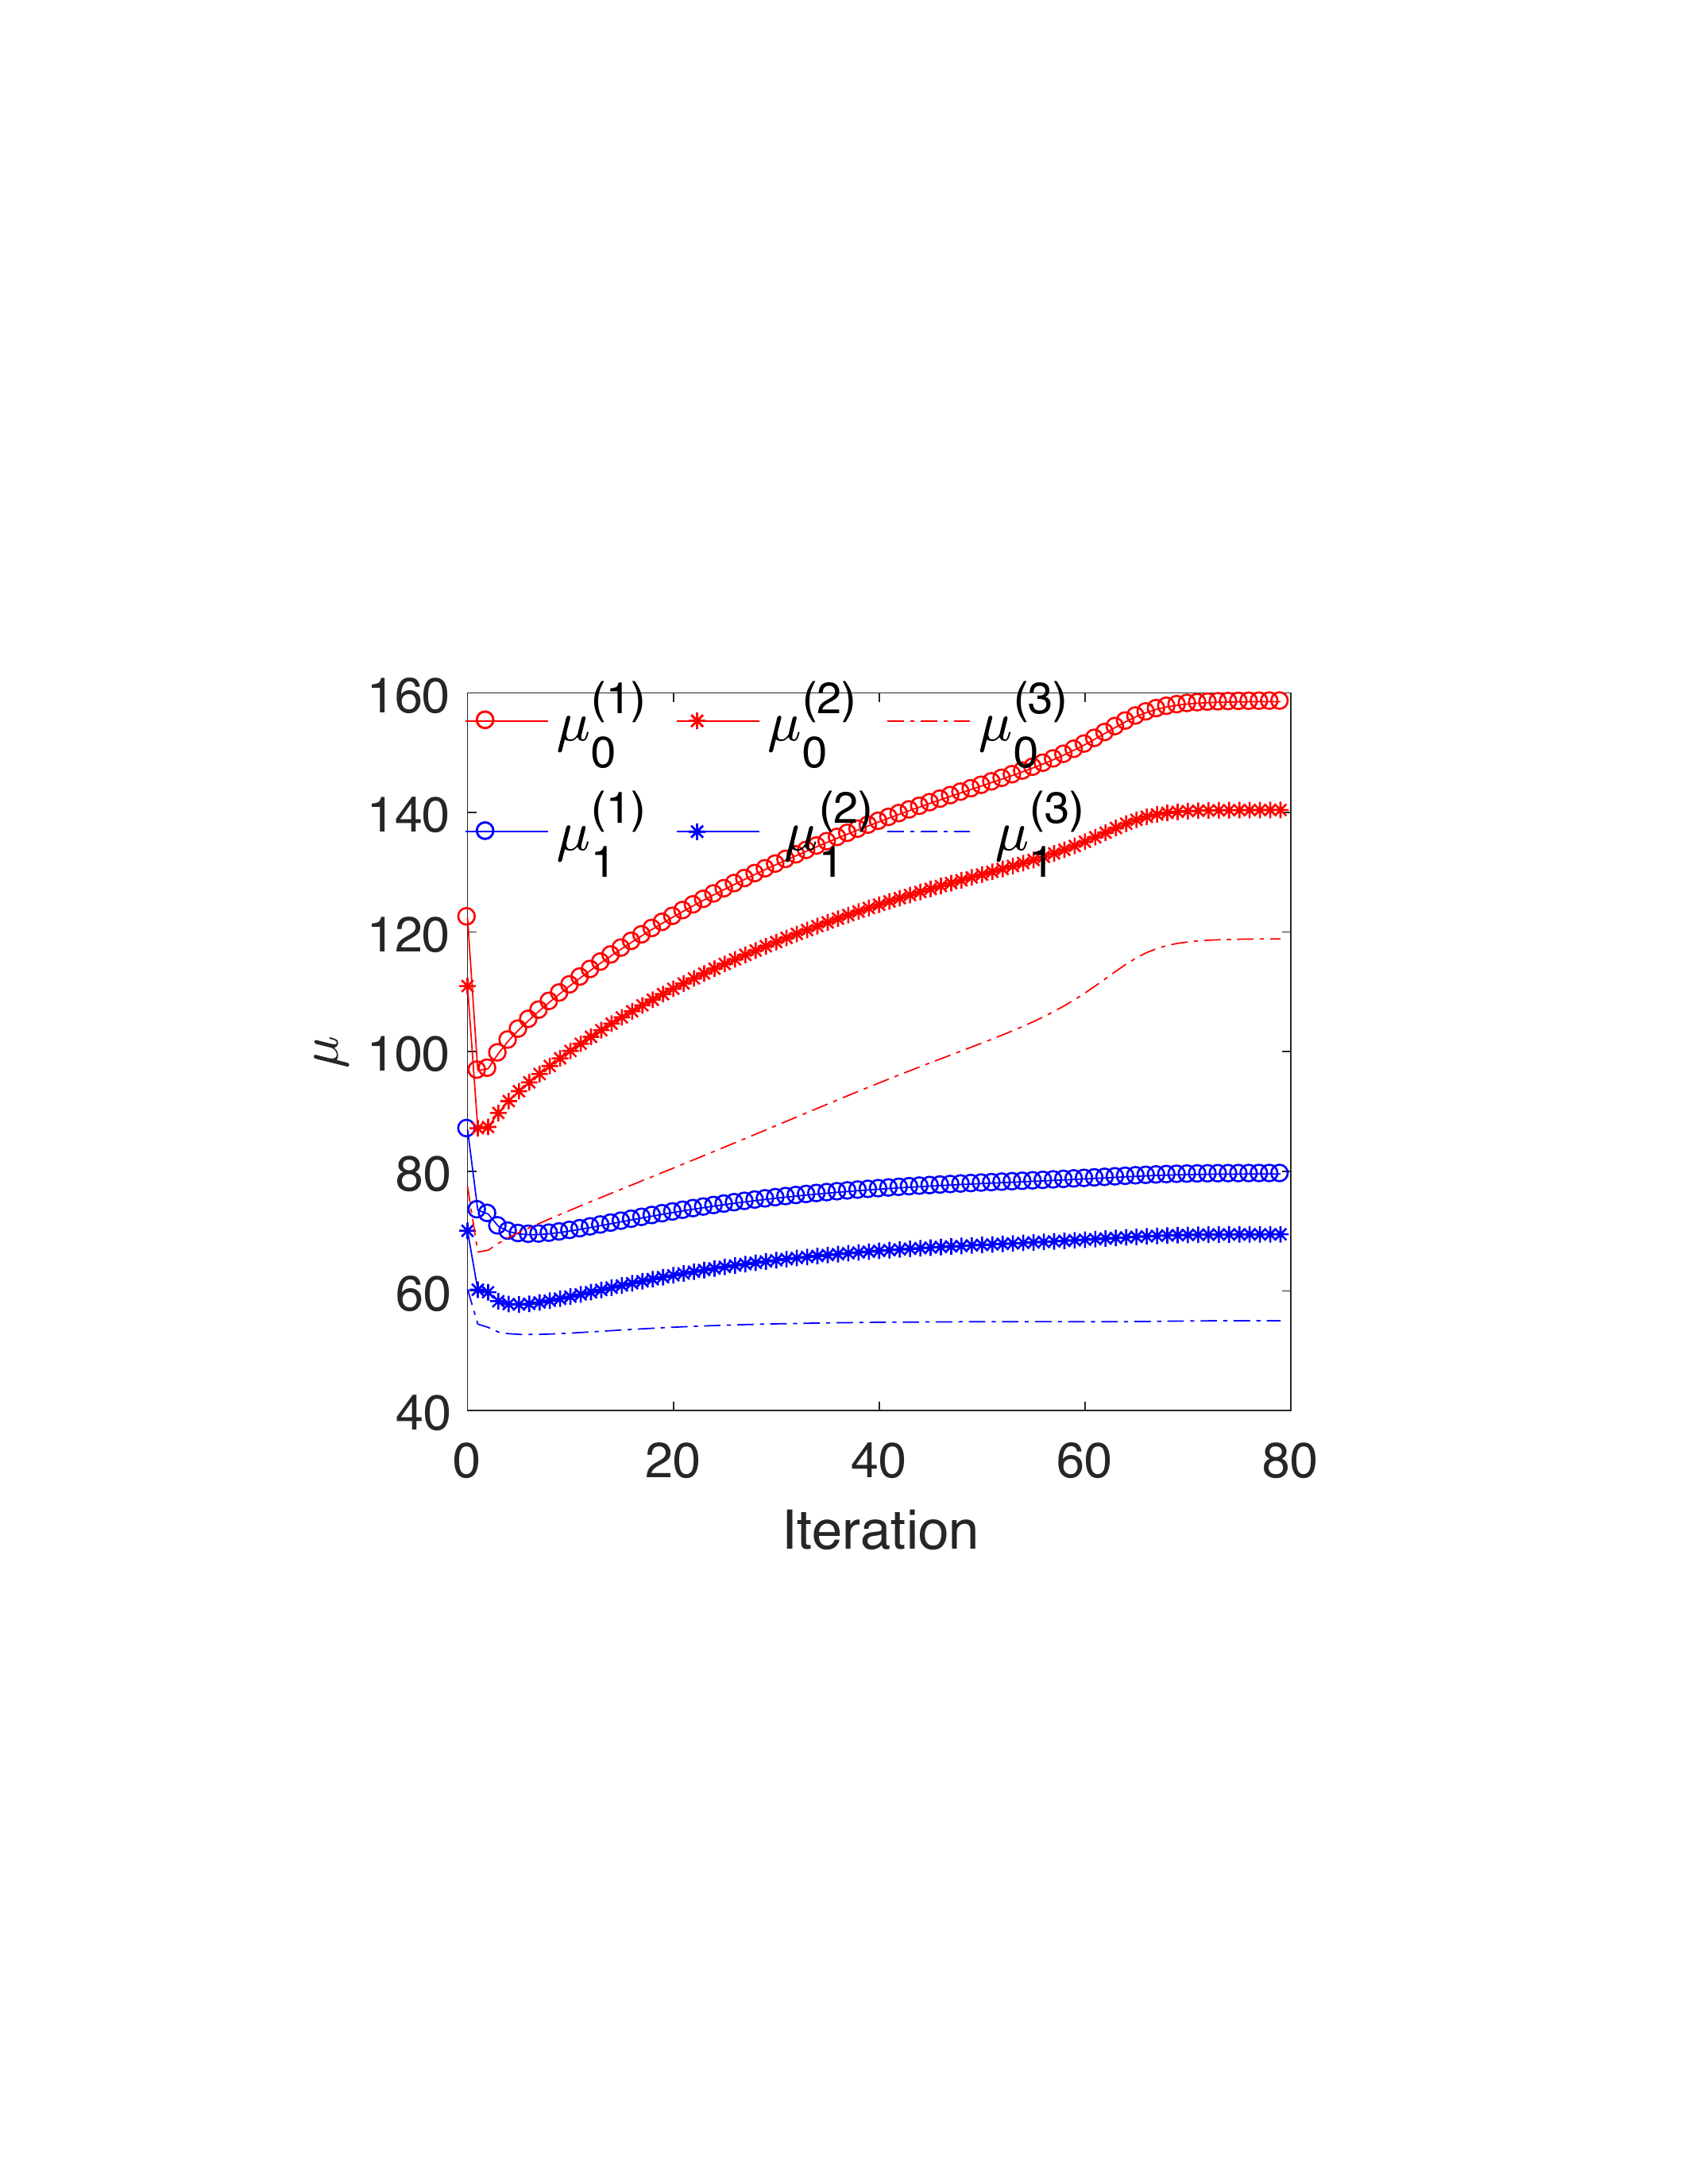}
}
\subfloat[Iterations of parameter $\boldsymbol{\Sigma}$]{%
      \includegraphics[height=1.7in,width=1.8in]{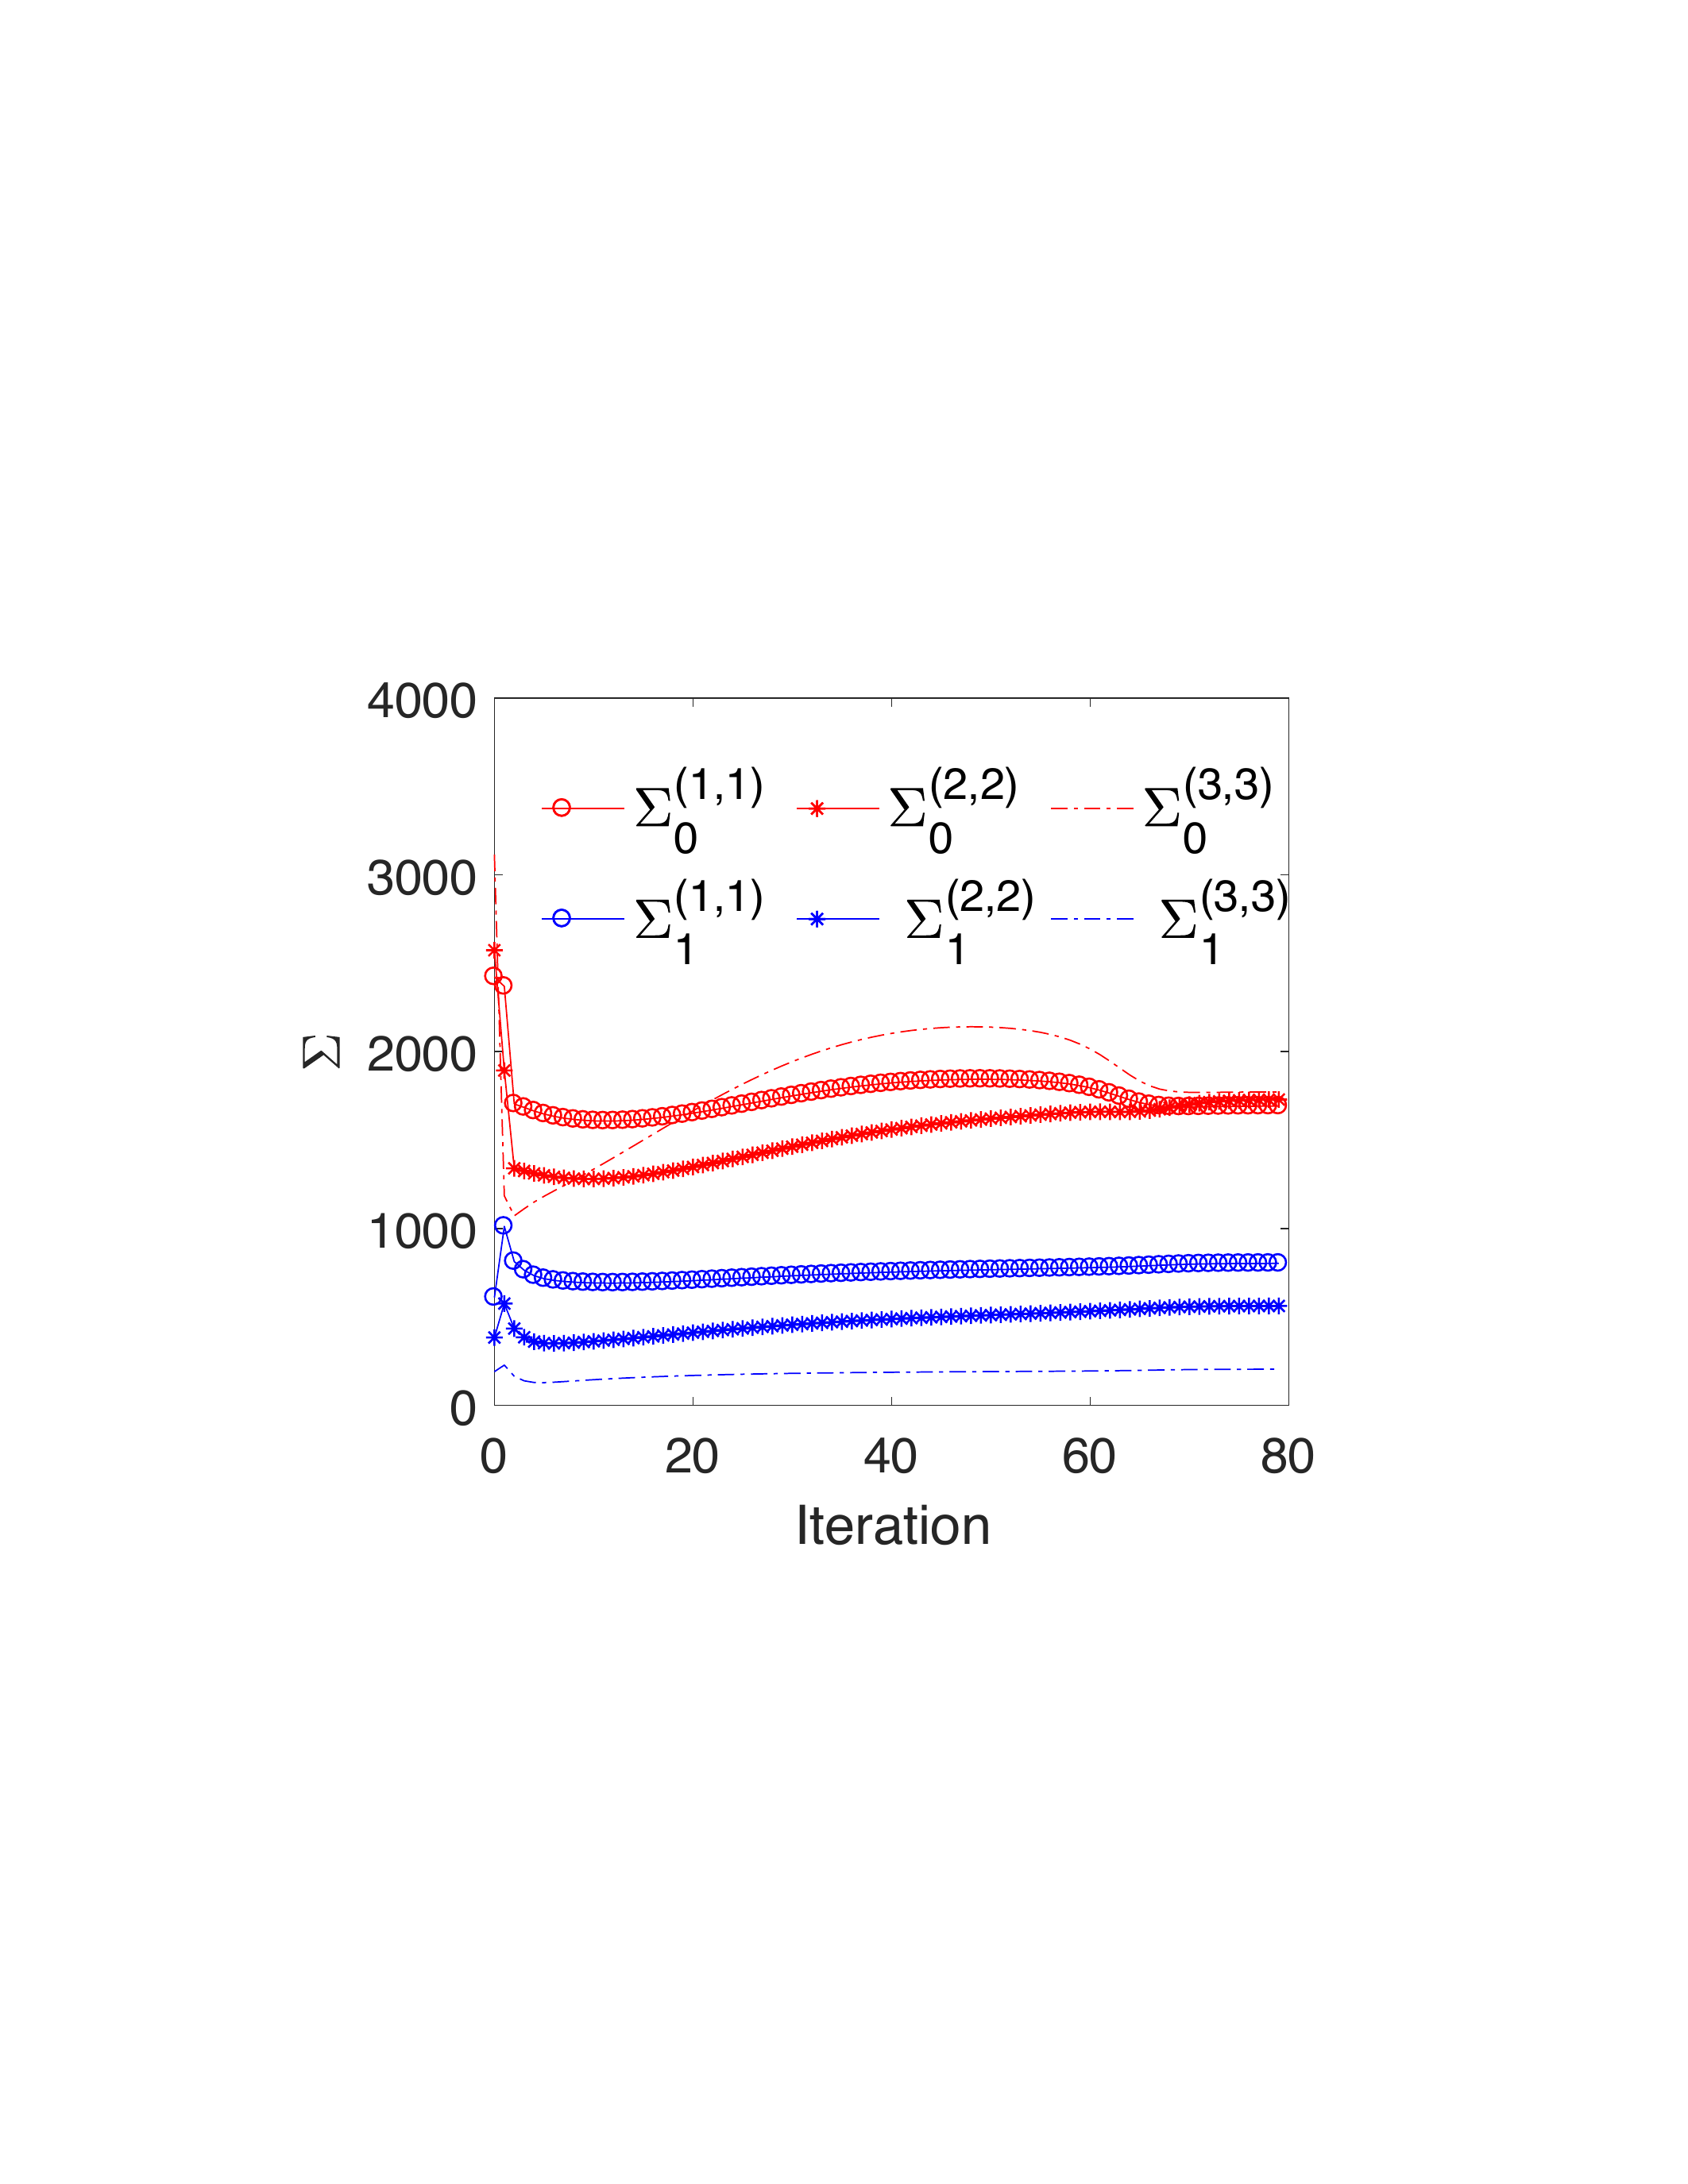}
}
\caption{Parameter iterations and convergence for unstructured EM without elevation feature}
\label{fig:EMNOElevmuSigmaap}
\end{figure}
\begin{figure}[ht]
\centering
\subfloat[Iteration of parameter $\boldsymbol{\mu}$]{%
      \includegraphics[height=1.8in,width=1.8in]{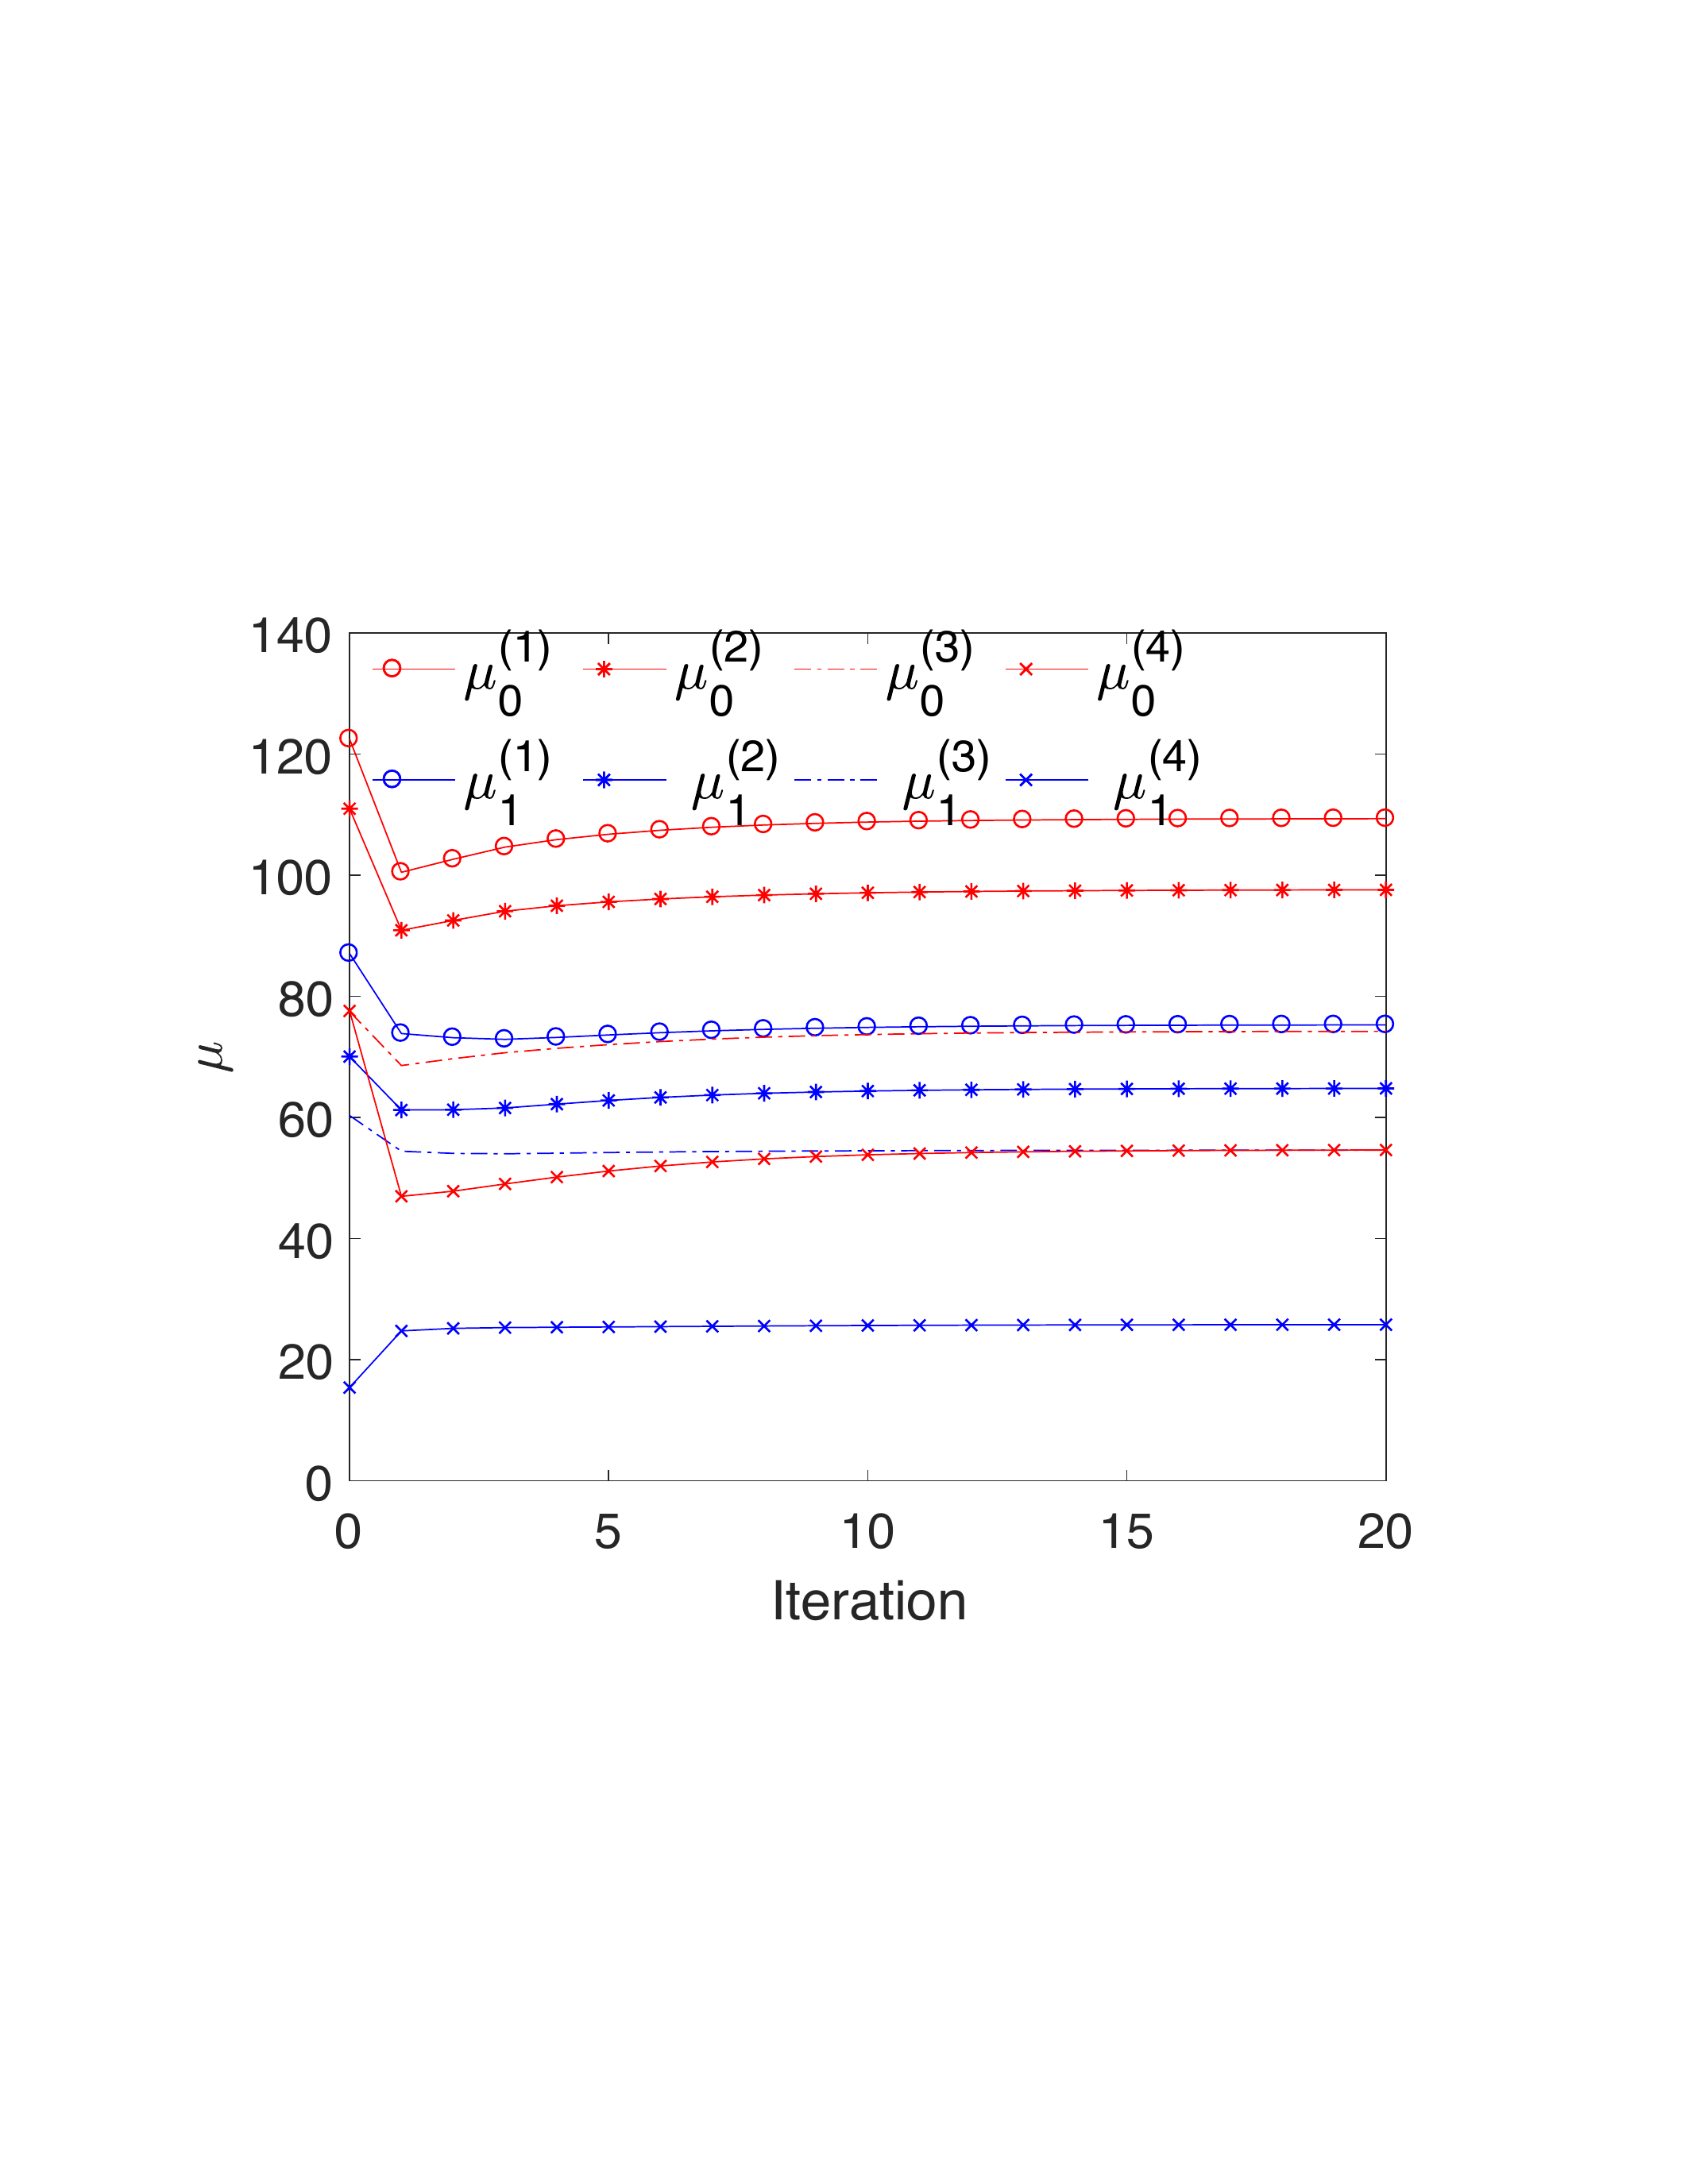}
}
\subfloat[Iterations of parameter $\boldsymbol{\Sigma}$]{%
      \includegraphics[height=1.8in,width=1.8in]{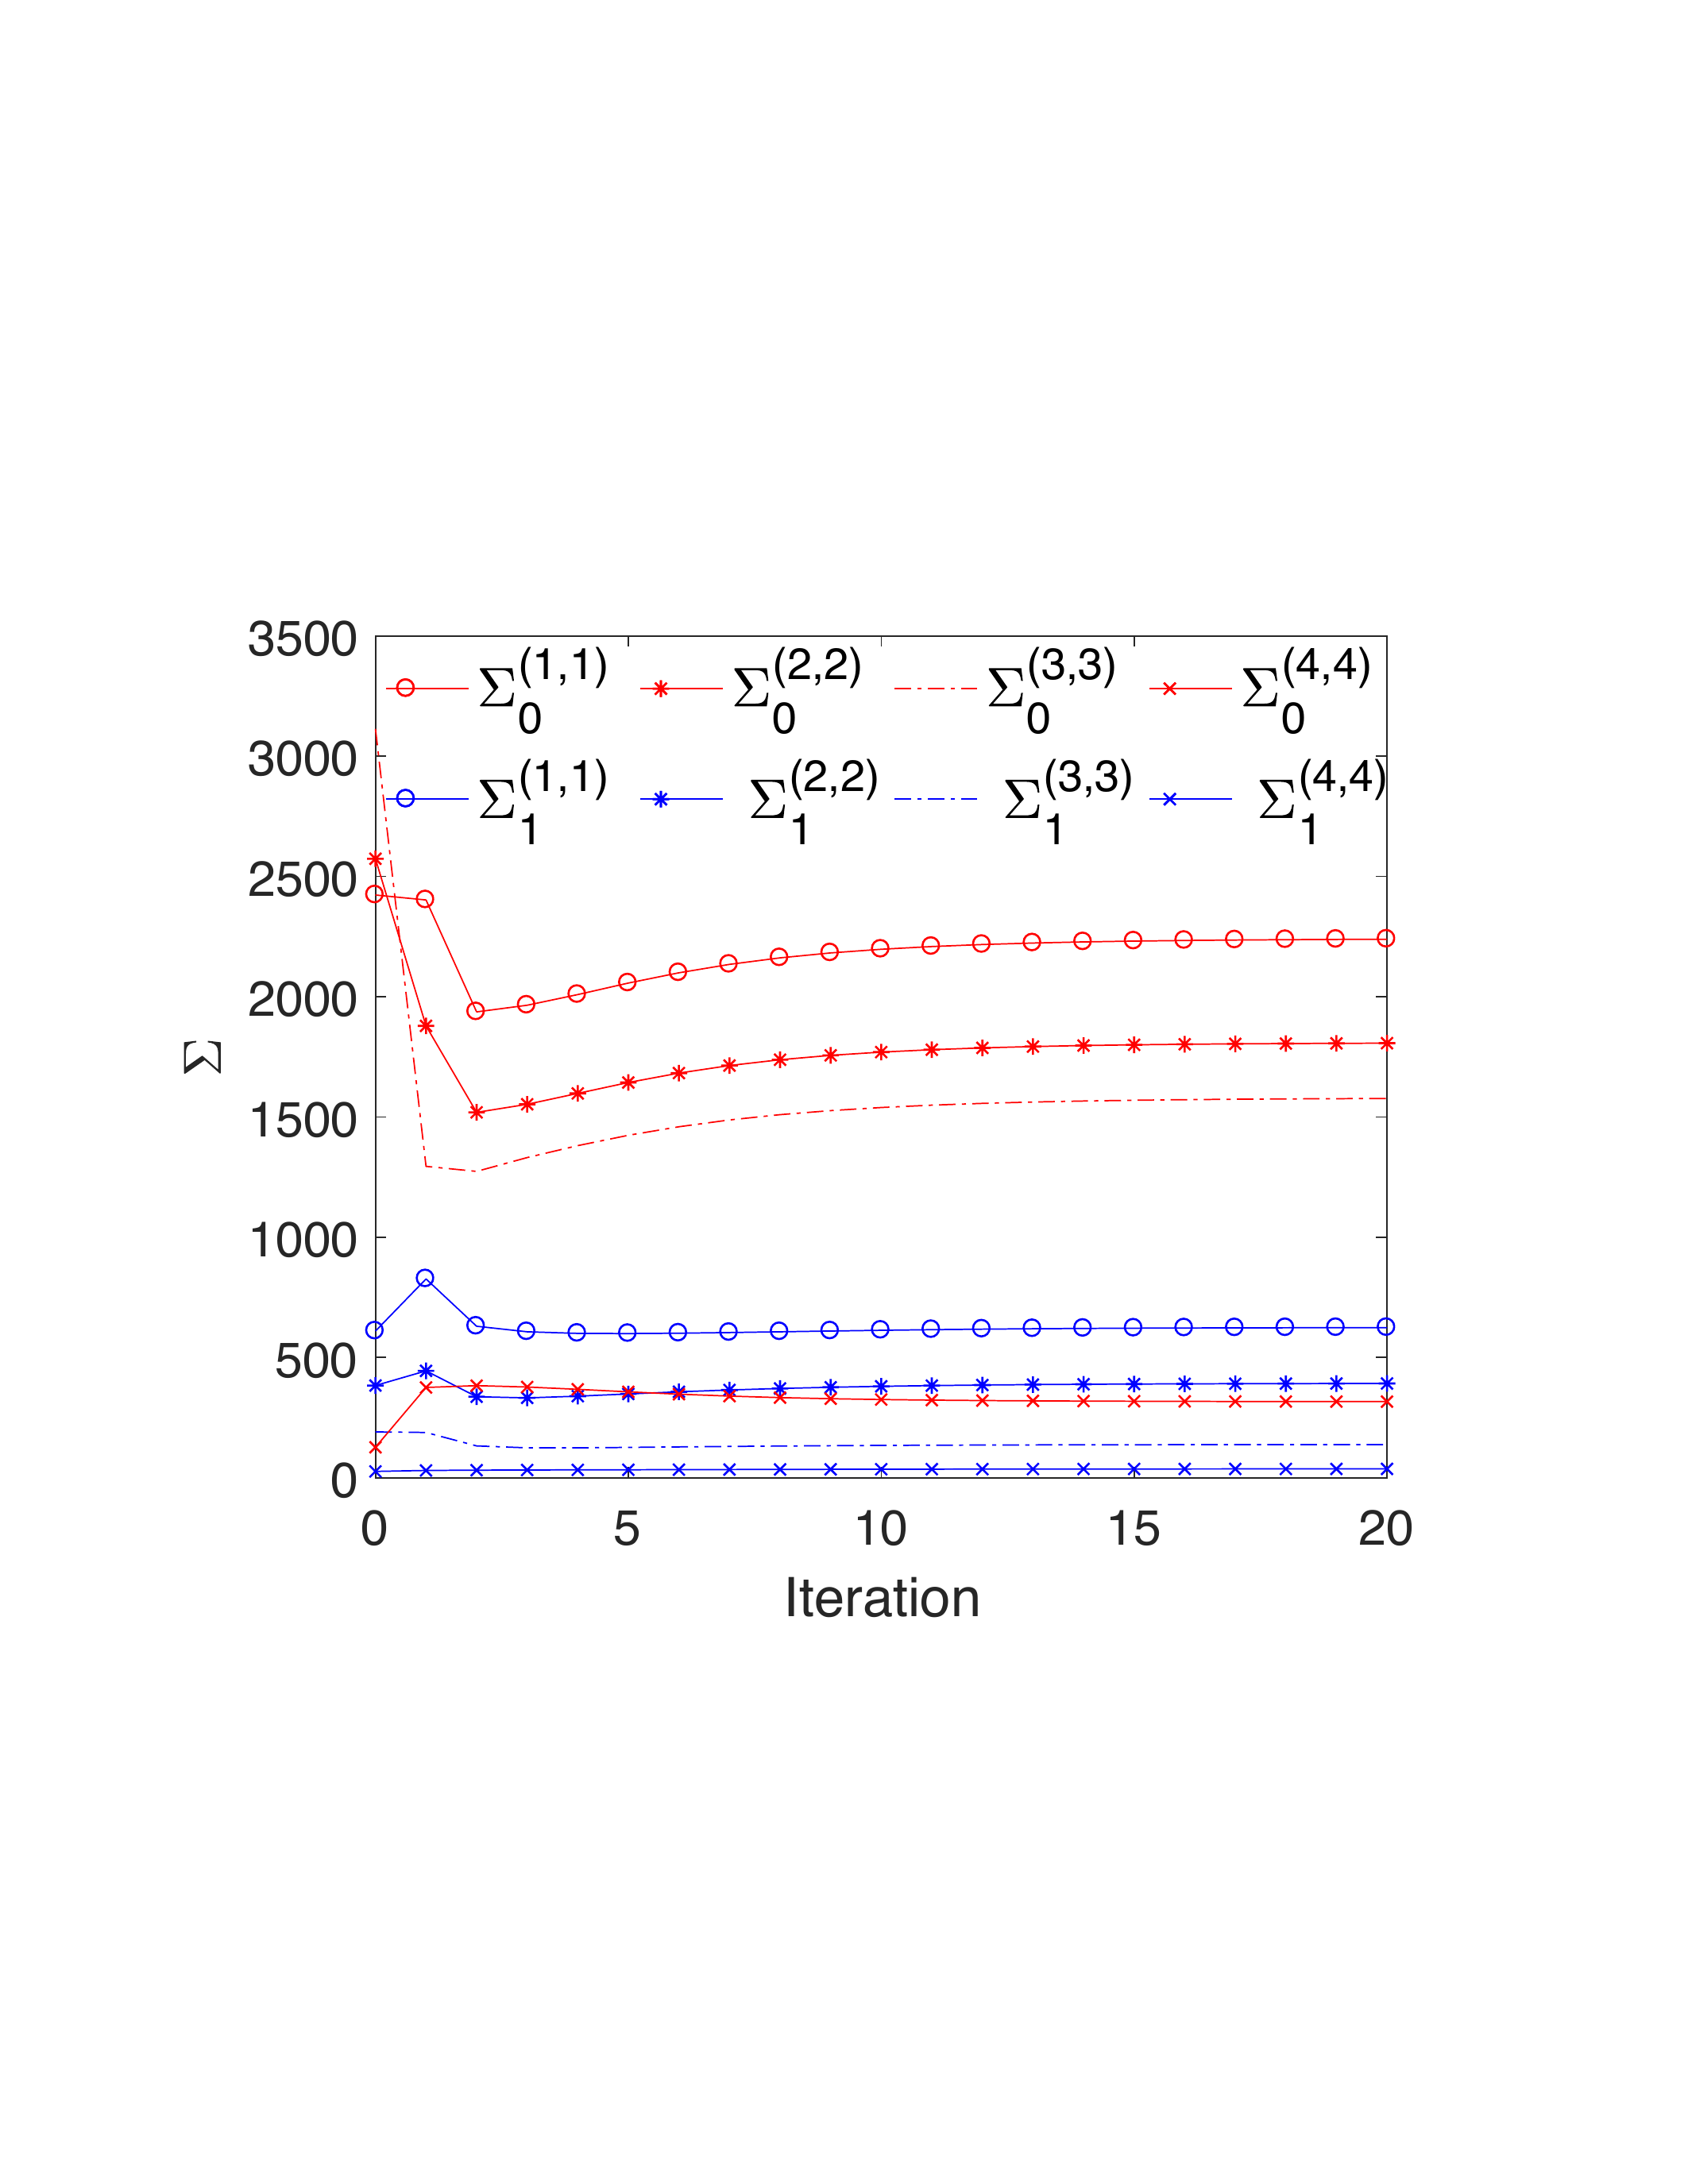}
}
\caption{Parameter iterations and convergence for unstructured EM with elevation feature}
\label{fig:EMmuSigmaap}
\end{figure}
\begin{figure}[ht]
\centering
\subfloat[Iteration of parameter $\boldsymbol{\mu}$]{%
      \includegraphics[height=1.7in,width=1.8in]{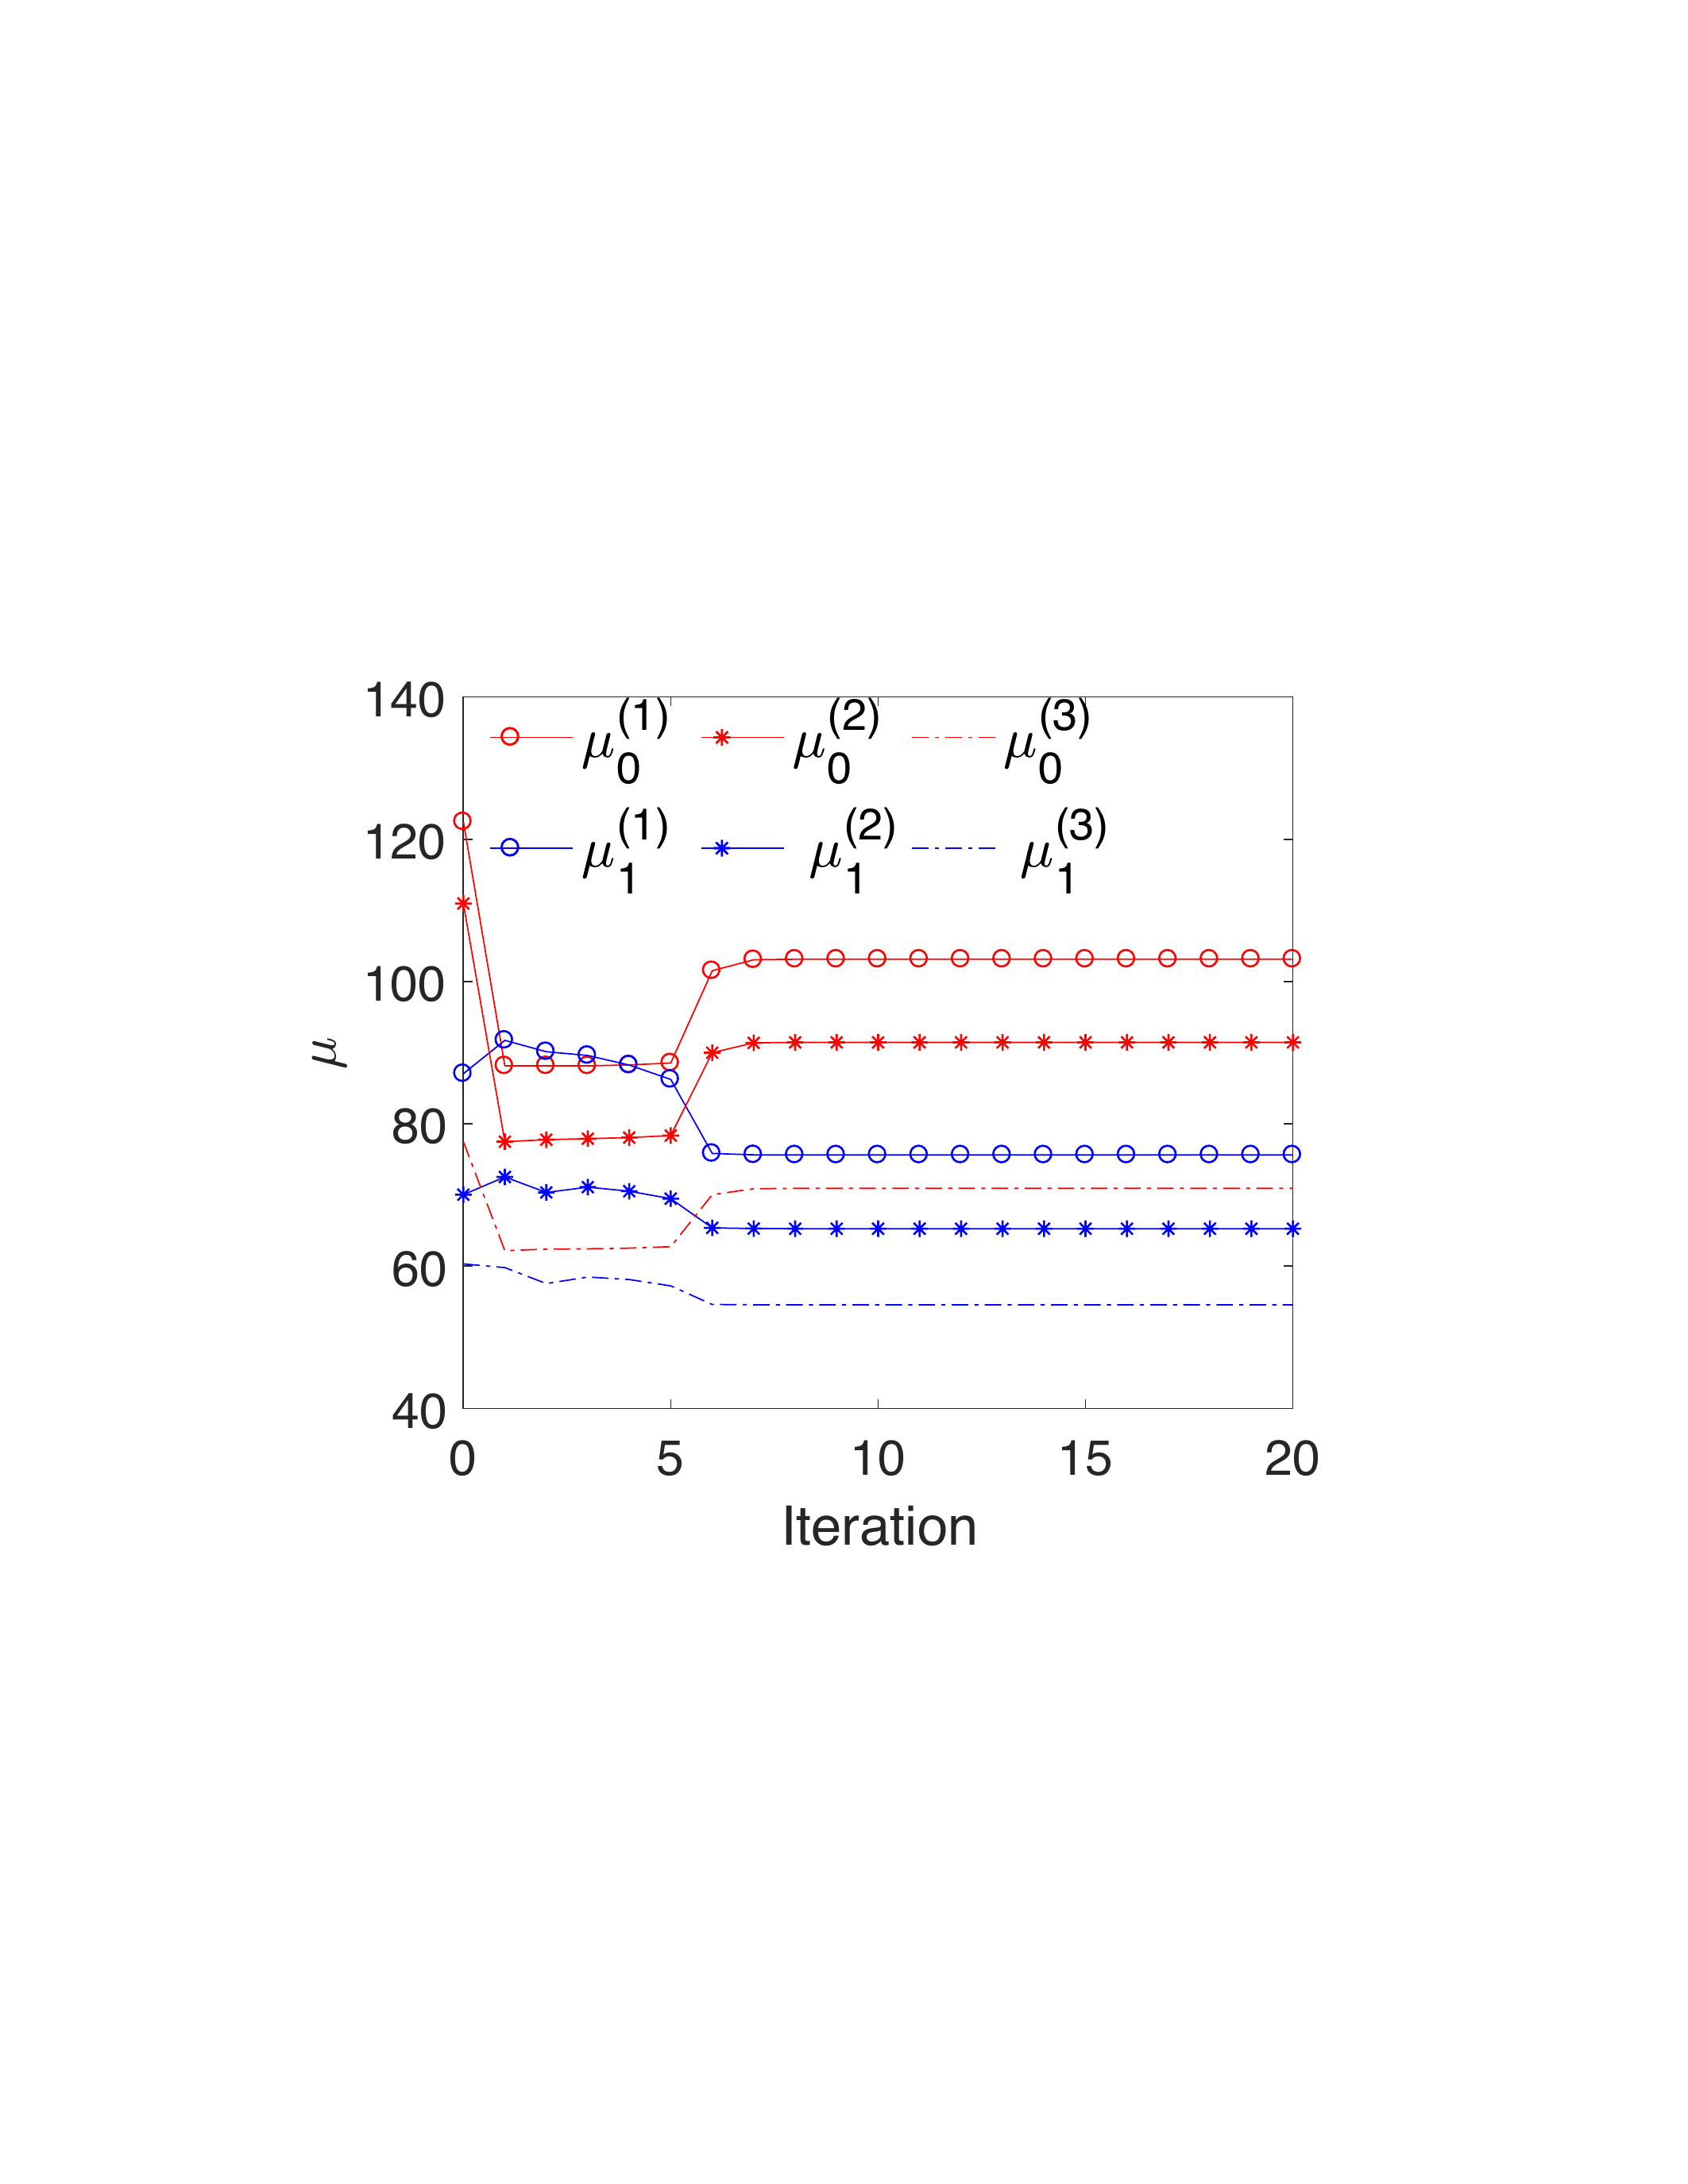}
}
\subfloat[Iterations of parameter $\boldsymbol{\Sigma}$]{%
      \includegraphics[height=1.7in,width=1.8in]{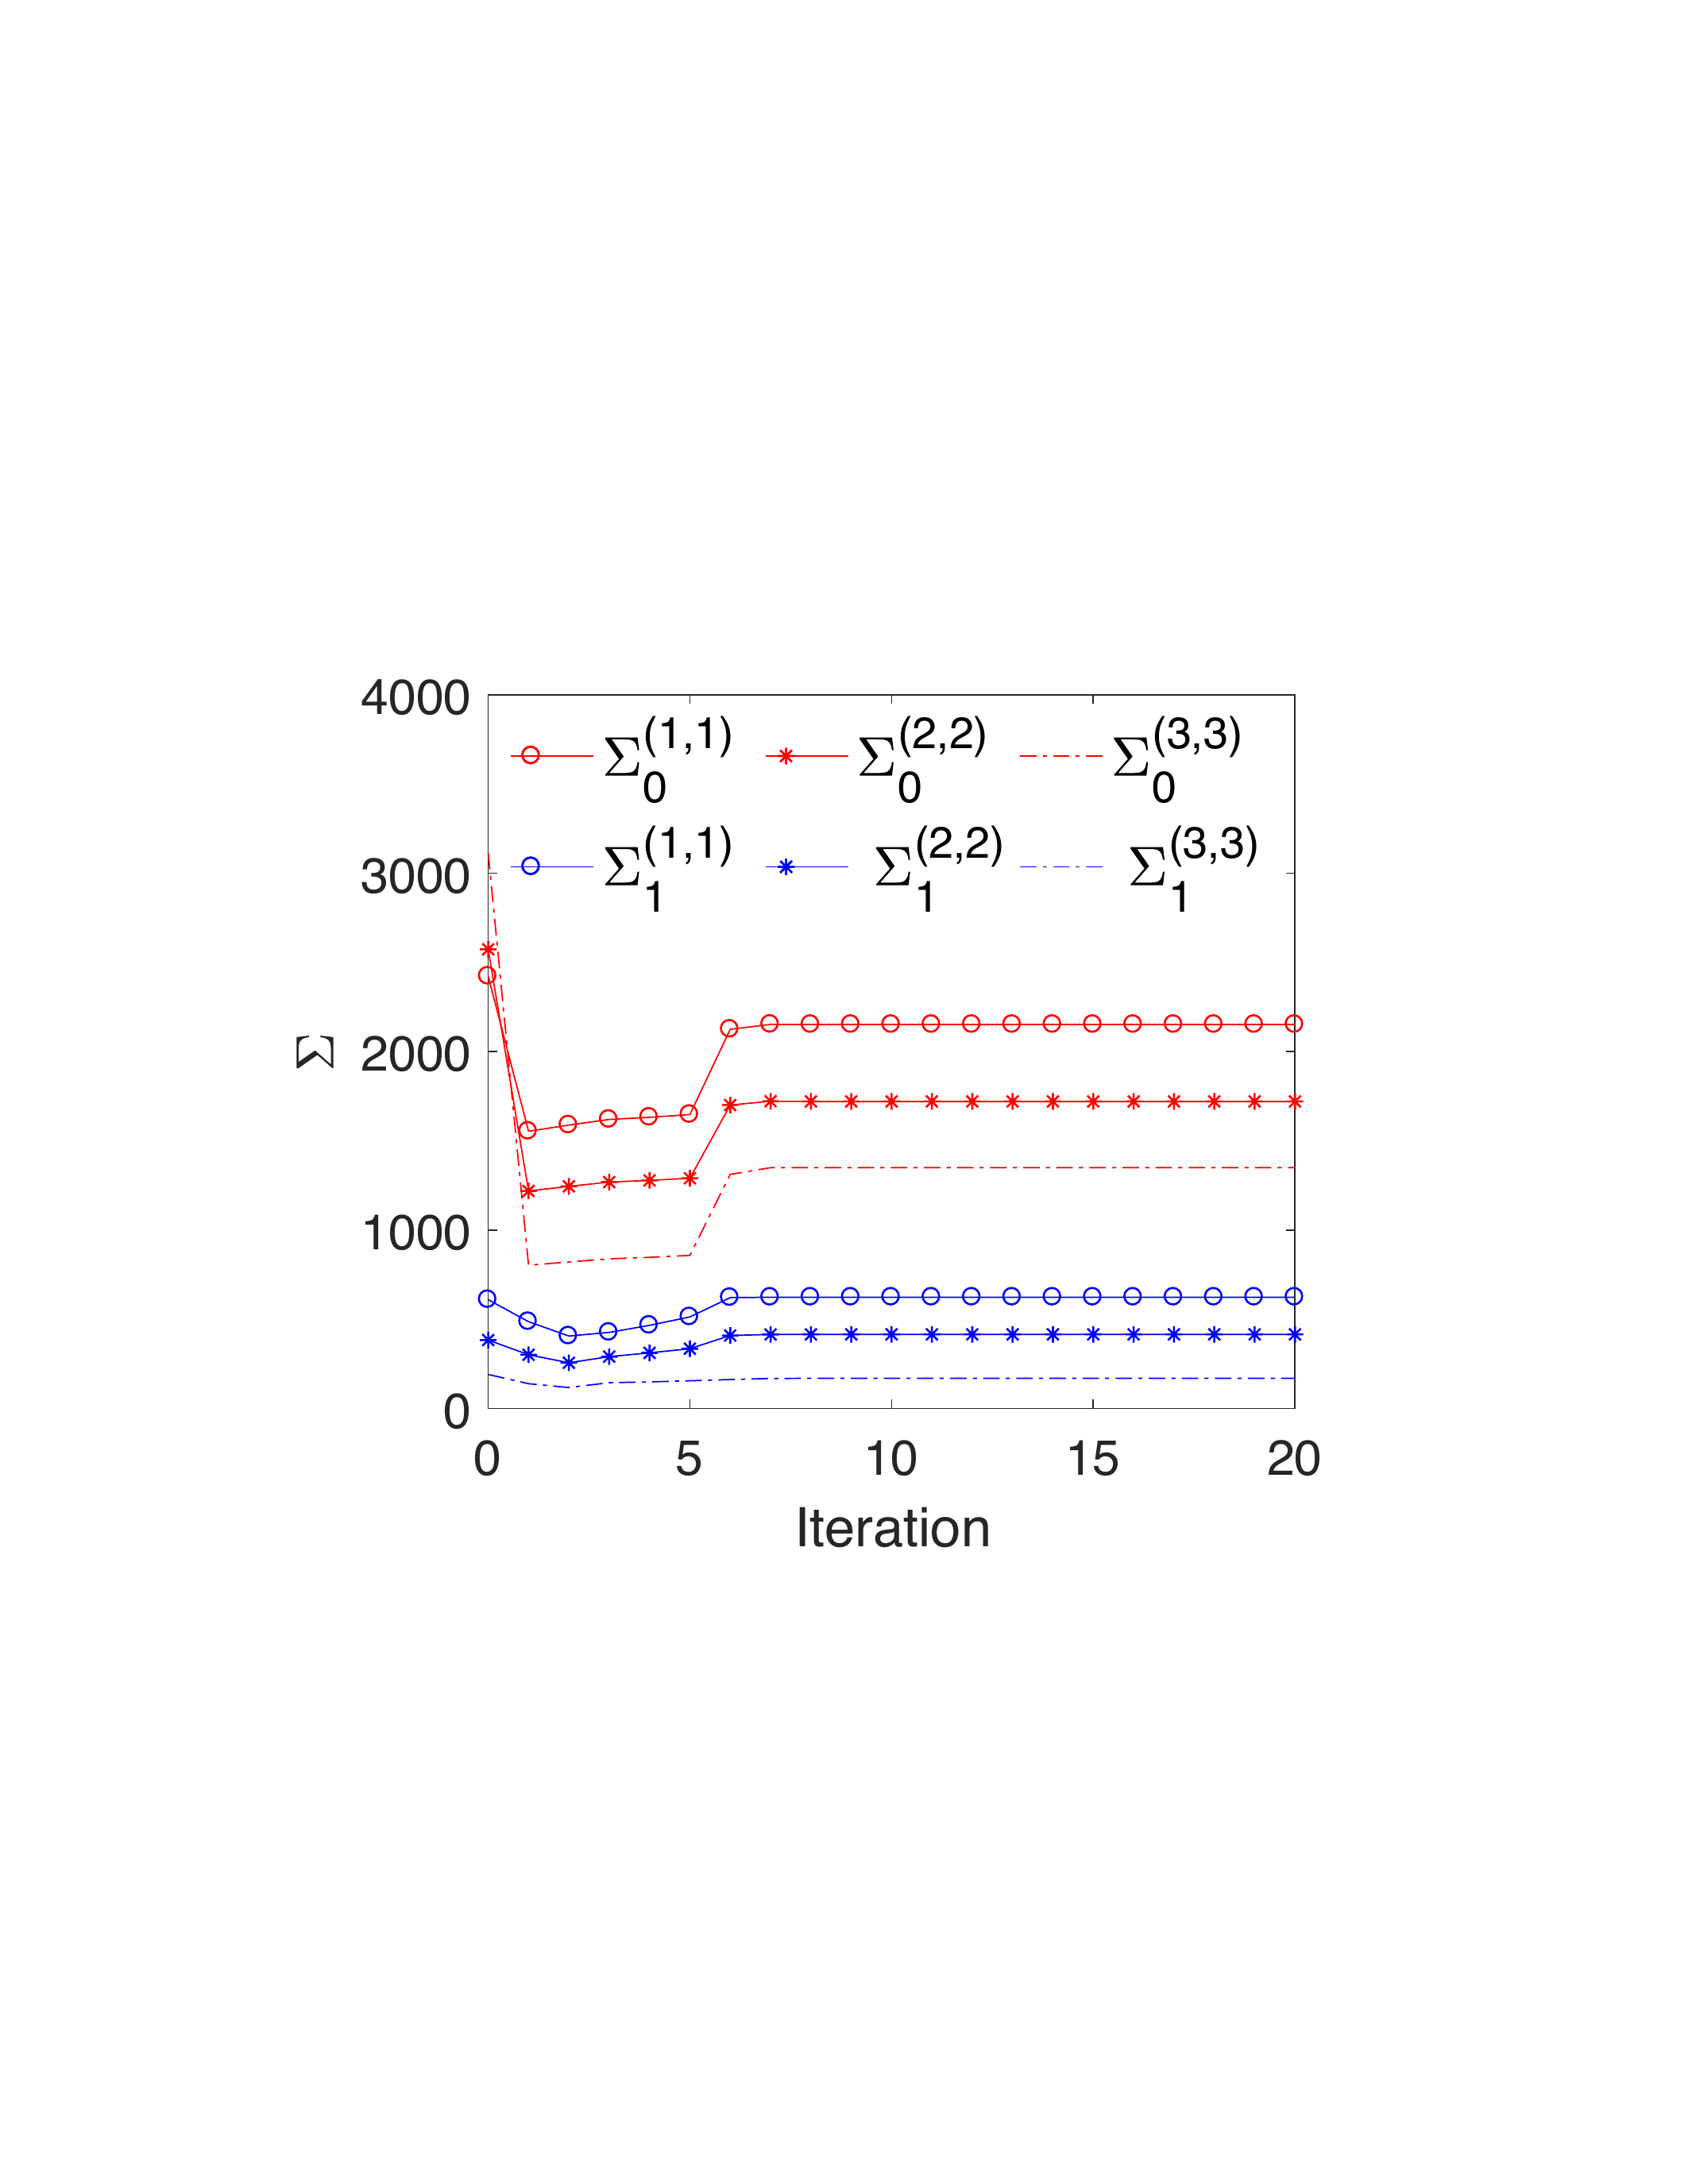}
}
\caption{Parameter iterations and convergence for structured EM algorithm}
\label{fig:HMTmuSigmaap}
\end{figure}

\begin{table}[ht]\footnotesize
\centering
\caption{Comparison on Mathew, Kinston flood data}
\label{tab:comp1ap}
\begin{tabular}{cccccc}
\hline
Classifiers & Class & Prec. &Recall & F & Avg. F\\ \hline
\multirow{2}{*}{EM i.i.d.(Converged) }&Dry&{0.91}&{0.18}&{0.30}&\multirow{2}{*}{0.51}\\ 
 &Flood&{0.55}&{0.98}&{0.70}&\\ \hline
 \multirow{2}{*}{EM i.i.d.(20 iterations) }&Dry&{0.83}&{0.51}&{0.63}&\multirow{2}{*}{0.70}\\ 
 &Flood&{0.65}&{0.89}&{0.76}&\\ \hline
\multirow{2}{*}{EM i.i.d.+ elev.}&Dry&{0.96}&{0.81}&{0.88}&\multirow{2}{*}{0.89}\\ 
 &Flood&{0.84}&{0.96}&{0.90}&\\ \hline 
\multirow{2}{*}{EM-Structure}&Dry&{0.94}&{0.99}&{0.96}&\multirow{2}{*}{0.96}\\ 
 &Flood&{0.99}&{0.94}&{0.96}&\\ \hline  
\end{tabular}
\end{table}

\begin{figure}[ht]
\centering
\subfloat[EM i.i.d. 20 iterations]{%
\includegraphics[height=2in]{figures/TC4EMNOElevClassificationNOEle20Iterations.pdf} 
}
\subfloat[EM i.i.d. 80 iterations]{%
\includegraphics[height=2in]{figures/TC4EMNOElevClassificationNOEle90Iterations.pdf} 
} \\
\subfloat[EM i.i.d. + elev.]{%
    \includegraphics[height=2in]{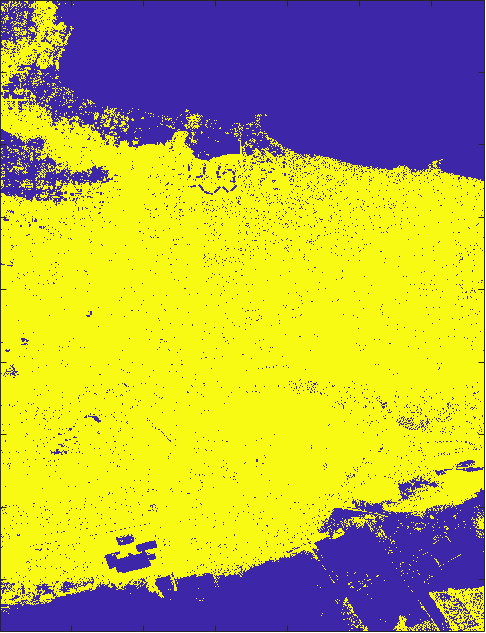} 
    }
\subfloat[EM with structure]{%
    \includegraphics[height=2in]{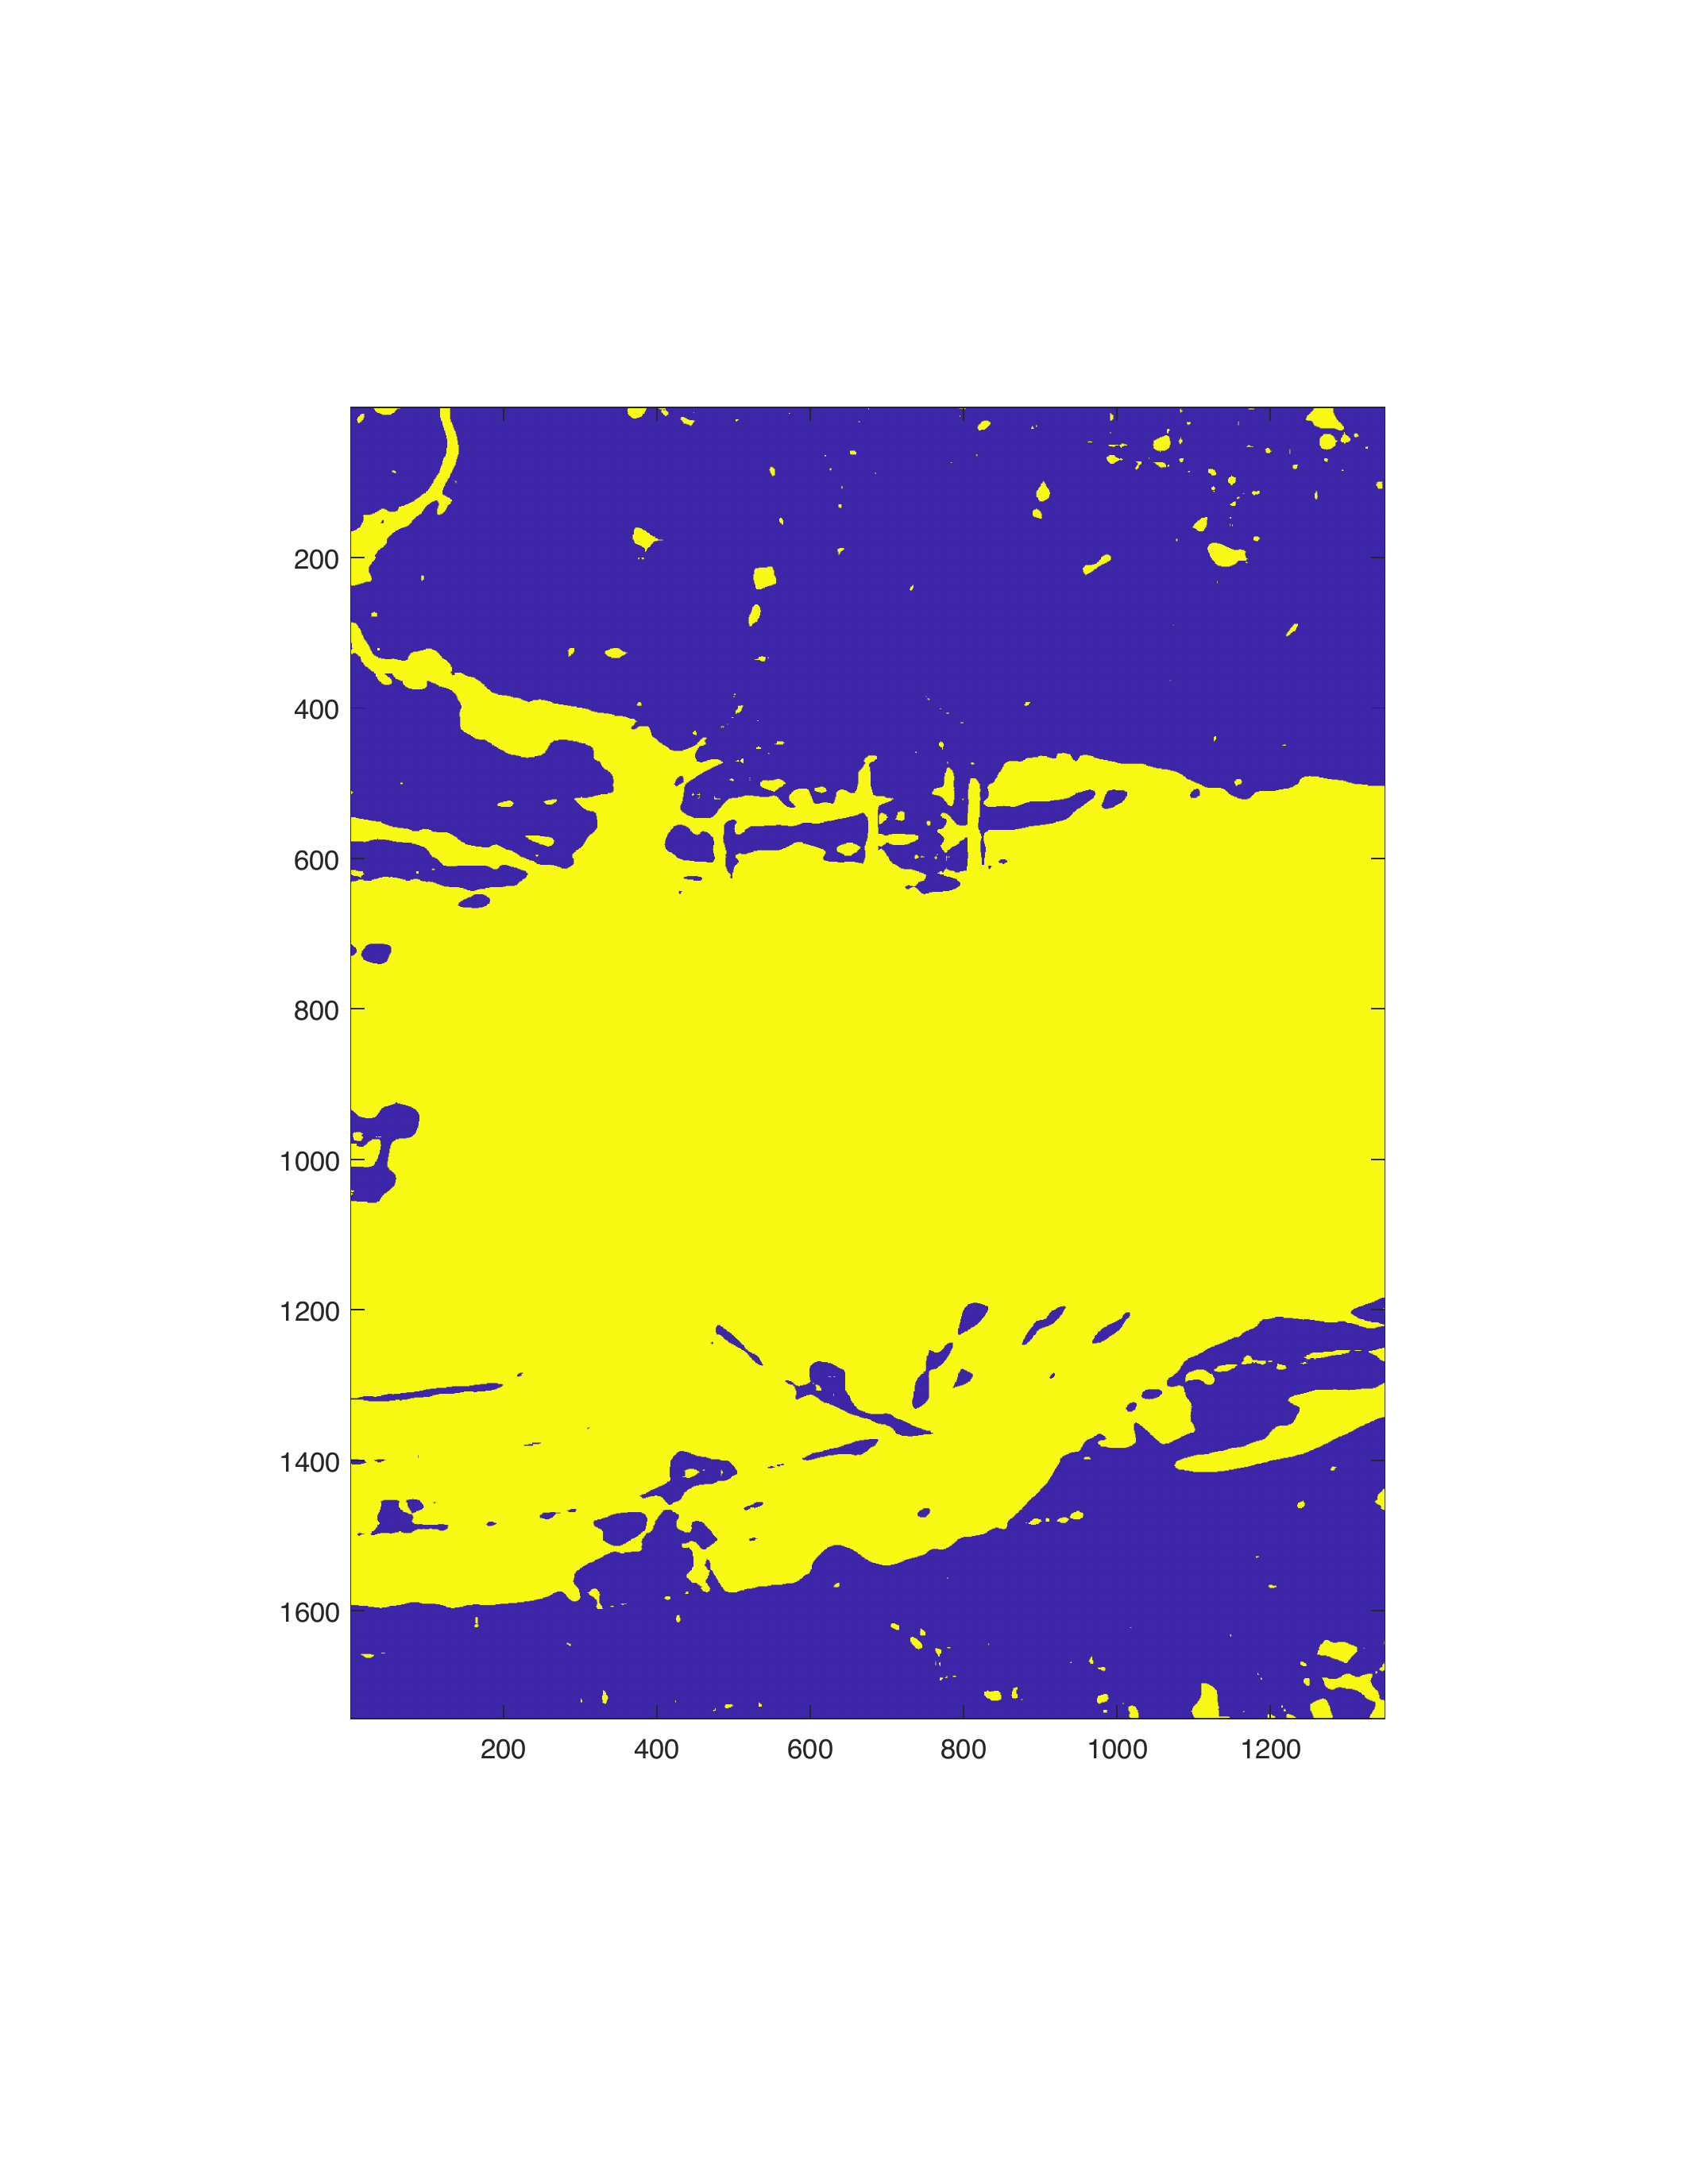} 
    }
\caption{Prediction result}
\label{fig:predresultap}
\end{figure}

% \subsection{Posterior Probability}

\begin{figure*}
\centering
\subfloat[]{%
      \includegraphics[height=1.4in]{figures/TC4EMNOElevMarginalProb0Iter.png}
}
\subfloat[]{%
      \includegraphics[height=1.4in]{figures/TC4EMNOElevMarginalProb1Iter.png}
}
\subfloat[]{%
      \includegraphics[height=1.4in]{figures/TC4EMNOElevMarginalProb5Iter.png}
}
\subfloat[]{%
      \includegraphics[height=1.4in]{figures/TC4EMNOElevMarginalProb10Iter.png}
}
\subfloat[]{%
      \includegraphics[height=1.4in]{figures/TC4EMNOElevMarginalProb20Iter.png}
}
\subfloat[]{%
      \includegraphics[height=1.4in]{figures/TC4EMNOElevMarginalProb80Iter.png}
}
\caption{Posterior Probability of Unstructured EM without elevation}
\label{fig:EMNOelevPosterProbap}
\end{figure*}

\begin{figure*}
\centering
\subfloat[]{%
      \includegraphics[height=1.4in]{figures/TC4EMMarginalProb0Iter.png}
}
\subfloat[]{%
      \includegraphics[height=1.4in]{figures/TC4EMMarginalProb1Iter.png}
}
\subfloat[]{%
      \includegraphics[height=1.4in]{figures/TC4EMMarginalProb2Iter.png}
}
\subfloat[]{%
      \includegraphics[height=1.4in]{figures/TC4EMMarginalProb5Iter.png}
}
\subfloat[]{%
      \includegraphics[height=1.4in]{figures/TC4EMMarginalProb15Iter.png}
}
\subfloat[]{%
      \includegraphics[height=1.4in]{figures/TC4EMMarginalProb20Iter.png}
}
\caption{Posterior Probability of Unstructured EM with elevation}
\label{fig:EMwithelevPosterProbap}
\end{figure*}

\begin{figure*}[h]
\centering
\subfloat[]{%
      \includegraphics[height=1.4in]{figures/TC4HMTMarginalProb0Iter.png}
}
\subfloat[]{%
      \includegraphics[height=1.4in]{figures/TC4HMTMarginalProb1Iter.png}
}
\subfloat[]{%
      \includegraphics[height=1.4in]{figures/TC4HMTMarginalProb5Iter.png}
}
\subfloat[]{%
      \includegraphics[height=1.4in]{figures/TC4HMTMarginalProb6Iter.png}
}
\subfloat[]{%
      \includegraphics[height=1.4in]{figures/TC4HMTMarginalProb10Iter.png}
}
\subfloat[]{%
      \includegraphics[height=1.4in]{figures/TC4HMTMarginalProb20Iter.png}
}
\caption{Posterior Probability of structured EM}
\label{fig:HMTPosterProbap}
\end{figure*}

% \subsection{Prediction result}
